# Supplementary material for: Interaction-Driven Filling-Induced Metal-Insulator Transitions in 2D Moir\'e Lattices
Source: arXiv:2012.04554 source file (2021-08-24)
Supplement: Supplementary file 1 [file SM.pdf]

# Supplemental Materials for "Interaction-Driven Filling-Induced Metal-Insulator Transitions in 2D Moiré Lattices"

Haining Pan and Sankar Das Sarma
*Condensed Matter Theory Center and Joint Quantum Institute,*
*Department of Physics, University of Maryland, College Park, Maryland 20742, USA*

## PERTURBATIVE METHOD

We start with the Hubbard model in Eq.(1) in the main text. The kinetic term $H_0$ in the momentum space is

$$H_0 = \sum_s \sum_{\boldsymbol{k}\in\mathbb{BZ}} \varepsilon_s(\boldsymbol{k}) c_{\boldsymbol{k},s}^\dagger c_{\boldsymbol{k},s}, \tag{1}$$

where $\boldsymbol{k}$ is summed over the first Brillouin zone ($\mathbb{BZ}$) of the moiré lattice, and $\varepsilon_s(\boldsymbol{k})$ is the noninteracting energy which should reproduce the band structure of $WSe_2$ calculated from the continuum Hamiltonian in Ref. 1. The interaction term $H_1$ in the momentum space is

$$H_1 = \frac{1}{2\mathcal{N}} \sum_{s,s'} \sum_{\boldsymbol{k}\in\mathbb{BZ}} U(\boldsymbol{k}_\alpha - \boldsymbol{k}_\delta) \delta_{\boldsymbol{k}_\alpha,\boldsymbol{k}_\beta,\boldsymbol{k}_\gamma,\boldsymbol{k}_\delta} c_{\boldsymbol{k}_\alpha,s}^\dagger c_{\boldsymbol{k}_\beta,s'}^\dagger c_{\boldsymbol{k}_\gamma,s'} c_{\boldsymbol{k}_\delta,s}, \tag{2}$$

where $\mathcal{N}$ is the total number of sites in the lattice. Here the interaction in the momentum space is

$$U(\boldsymbol{q}) = \sum_i U(\boldsymbol{R}_i) e^{i\boldsymbol{q}\cdot\boldsymbol{R}_i}, \tag{3}$$

and the conservation of momentum is imposed by the Kronecker delta function

$$\delta_{\boldsymbol{k}_\alpha,\boldsymbol{k}_\beta,\boldsymbol{k}_\gamma,\boldsymbol{k}_\delta} = \sum_{\boldsymbol{G}} \delta(\boldsymbol{k}_\alpha + \boldsymbol{k}_\beta - \boldsymbol{k}_\gamma - \boldsymbol{k}_\delta, \boldsymbol{G}), \tag{4}$$

where $\boldsymbol{G}$ is any moiré reciprocal lattice vector.

The mean-field approximation can be obtained by applying the Wick's theorem to the interaction term, i.e.,

$$H_{\text{int}} = \frac{1}{\mathcal{N}} \sum_{s,s'} \sum_{\boldsymbol{k}} U(\boldsymbol{k}_\alpha - \boldsymbol{k}_\delta) \delta_{\boldsymbol{k}_\alpha,\boldsymbol{k}_\beta,\boldsymbol{k}_\gamma,\boldsymbol{k}_\delta} \left[ \left\langle c_{\boldsymbol{k}_\alpha,s}^\dagger c_{\boldsymbol{k}_\delta,s} \right\rangle c_{\boldsymbol{k}_\beta,s'}^\dagger c_{\boldsymbol{k}_\gamma,s'} - \left\langle c_{\boldsymbol{k}_\alpha,s}^\dagger c_{\boldsymbol{k}_\gamma,s'} \right\rangle c_{\boldsymbol{k}_\beta,s'}^\dagger c_{\boldsymbol{k}_\delta,s} \right]. \tag{5}$$

The interaction may break the discrete translational symmetry spontaneously and result in a charge density wave and spin density wave with a larger period than the original moiré unit cell. Therefore, we can construct a spin texture in the real space as the ansatz and feed it into the mean-field Hamiltonian to find a self-consistent solution iteratively. For example, at half-filling $\nu = 1$, the two completing ansätze, which can be stable insulating states at small $\epsilon$, are $120^\circ$ antiferromagnetic Néel state with an enlarged $\sqrt{3}\times\sqrt{3}$ unit cell, and ferromagnetic state with the original moiré lattice. We calculate the energies of both self-consistent states as a function of $\epsilon$ to determine the energy-favorable phase. This is the standard procedure to find the phase diagram in the moiré-Hubbard model, where more details can be found in the Supplemental Material in Ref. 2.

In this work, instead of solving at the exact fillings (e.g., $\nu = 1, 1/3$, etc.), we study the self-consistent solutions at the proximity of exact fillings by perturbation from the solution at exact filling. For example, at the proximity of half-filling ($\nu = 19/20, 14/15, 9/10, 21/20, 16/15, 11/10$ ), we still use the $120^\circ$ antiferromagnetic Néel state and the ferromagnetic state as we did at the exact half-filling. It turns out that, if the filling is not too far from the half-filling, these self-consistent solutions at exact half-filling still remain stable with the only difference being the change from insulating states to metallic states.

## RESULTS FOR THE PROXIMITY OF $\nu = 1/3$

In this section, we present the calculated charge gap as a function of $\epsilon$ for fixed $\theta = 4^\circ$ for several values of fillings that are close to 1/3 in Fig. 1.

At $\nu = 1/3$, the $120^\circ$ antiferromagnetic insulating state [AFI in Fig. 1(e)] is more energy-favorable at small $\epsilon$ with the completing state being the ferromagnetic insulating state [FMI in Fig. 1(d)] at $\epsilon < 30$ and ferromagnetic metallic state [FMM in Fig. 1(i)] at $30 < \epsilon < 33$. At large $\epsilon$, the ferromagnetic metallic state is more energy-favorable with the completing state being AFI at $33 < \epsilon < 43$, and $180^\circ$ antiferromagnetic metallic state [AFM in Fig. 1 (f)] at $\epsilon > 43$.

When the filling is perturbed from 1/3, we still use the FMI and AFI as the ansätze, and find that these

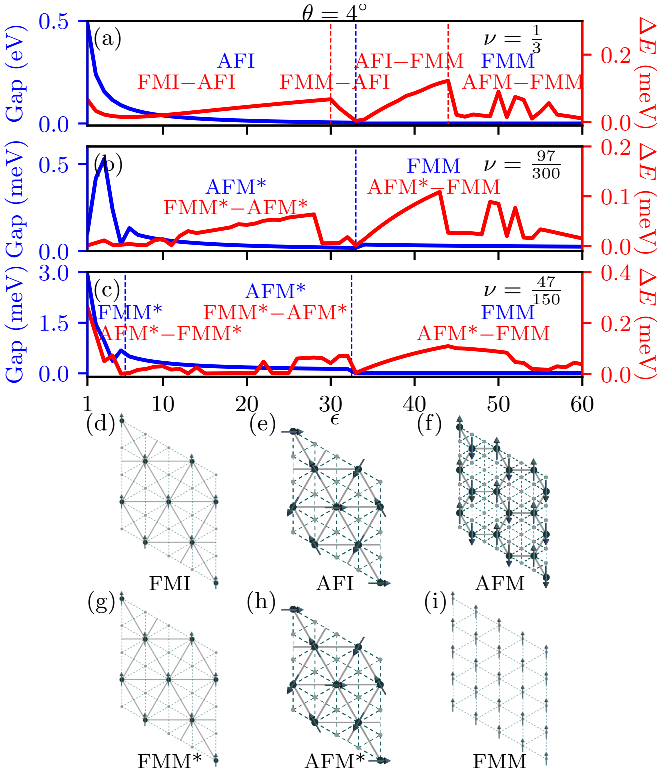


FIG. 1. The calculated charge gap (blue) as a function of $\epsilon$ for a fixed $\theta = 4^\circ$ at (a) $\nu = 1/3$; (b) $\nu = 97/300$; (c) $\nu = 47/150$. The red line is the absolute energy difference between two completing phases. The first order transition happens at the blue vertical dashed line with the name of phases labeled in blue. (d)-(i) show the real-space spin texture of each phase that can exist at $\nu = 1/3$ .

states remain self-consistent in the mean-field Hamiltonian. However, they have changed from insulating states into metallic states, namely, FMI in Fig. 1 (d) changes to FMM* in Fig. 1 (g), and AFI in Fig. 1 (e) changes to AFM* in Fig. 1 (h). From $\nu = 1/3$ to $\nu = 97/300$, as shown in Fig. 1 (b), the phase diagram does not change much: the spin textures remain the same while the antiferromagnetic insulating state becomes an antiferromagnetic metallic state. As the filling goes further away from 1/3, at $\nu = 47/150$ shown in Fig. 1 (c), we additionally find a ferromagnetic metallic state showing up at small $\epsilon$. All the states doped slightly below $\nu = 1/3$ are metallic states (note that the units of the charge gap are different), which manifests the metal-insulator transition driven by the fillings.

[1] H. Pan, F. Wu, and S. Das Sarma, Band topology, Hubbard model, Heisenberg model, and Dzyaloshinskii-Moriya interaction in twisted bilayer $WSe_2$, Phys. Rev. Research **2**, 033087 (2020).

[2] H. Pan, F. Wu, and S. Das Sarma, Quantum phase diagram of a Moiré-Hubbard model, Phys. Rev. B **102**, 201104 (2020).
